# Supplementary material for: Geometric effects in random assemblies of ellipses
Source: arXiv:1905.11777 ancillary file (2019-05-28)

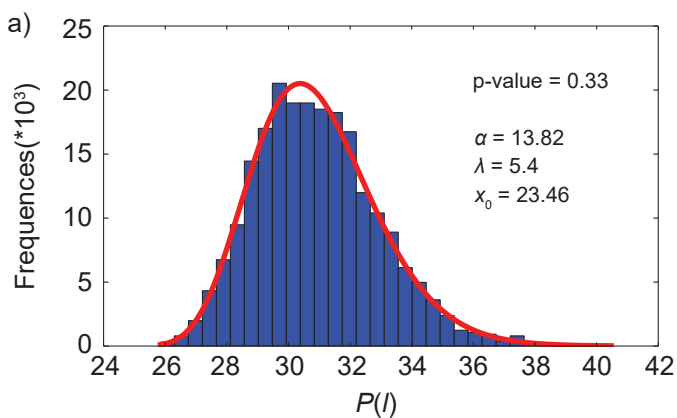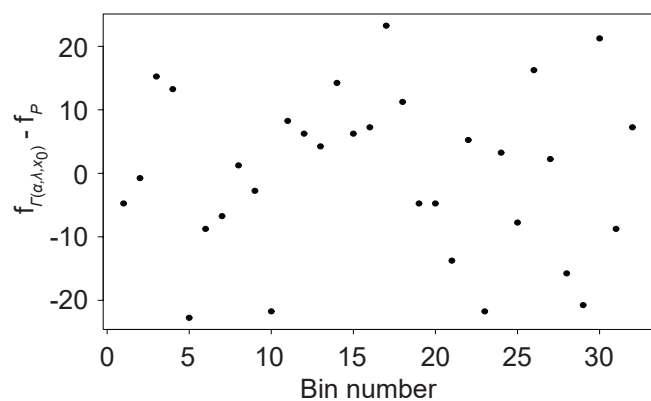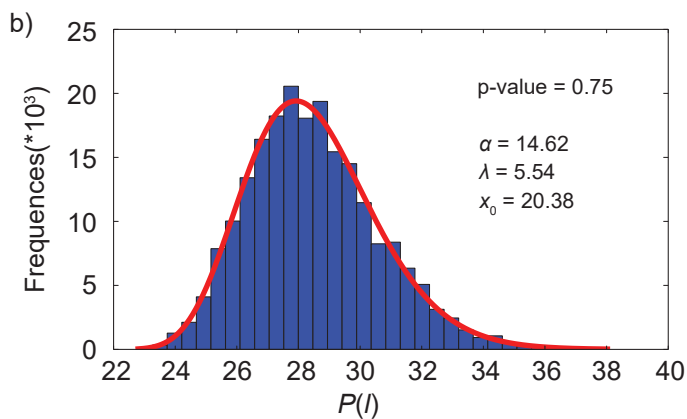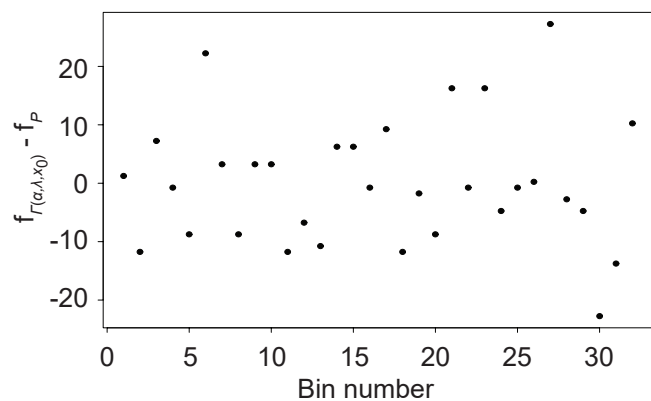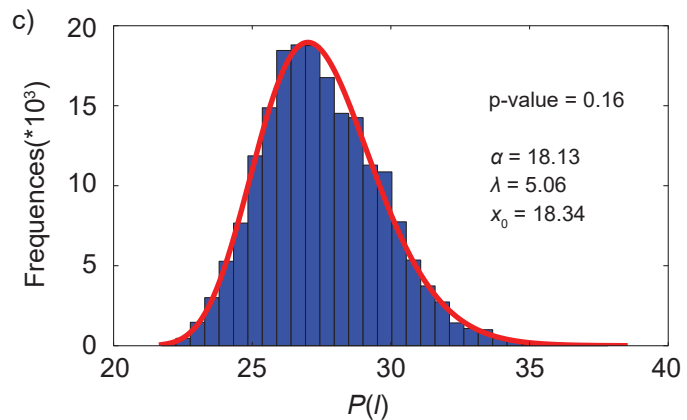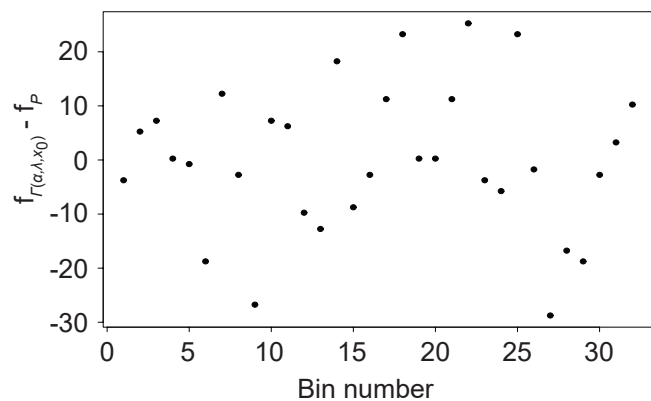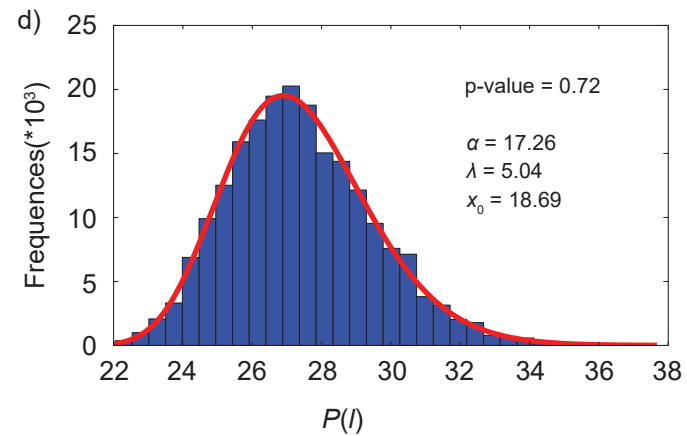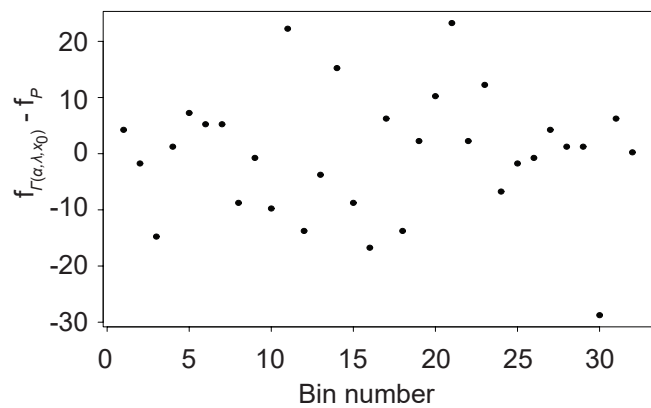

Supplement: Supplementary file 1 [file SIFig13.pdf]
